# Supplementary material for: From Dirichlet to Rubin: Optimistic Exploration in RL without Bonuses
Source: arXiv:2205.07704 source file (2022-06-22)
Supplement: Supplementary file 1 [file bayesian_bootstrap.tex]

%!TEX root = ../BayesUCBVI.tex
\section{Bayesian Bootstrap}
We denote by $\cB$ the set of distributions supported on the unit interval $[0,1]$ and by $E(\nu)  := \E_{X\sim\nu}[X]$ the mean of an element $\nu\in\cB$.

\paragraph{Frequentist non-parametric UCB}
A good quantity to measure the deviation of samples of $\nu$ from its mean is the minimal Kullback-Leibler divergence
\[
\Kinf(\nu,u) = \inf\left\{  \KL(\nu,\nu'): \nu'\in\cB, E(\nu) \geq u\right\}\,.
\]
Indeed we have the following deviation inequality
\begin{theorem} \label{th:ineq_kinf_anytime}
For all $\nu\in\cB$, for all $\delta\in[0,1]$, for i.i.d sample  $X_1,\ldots,X_n\sim \nu$ and the associated empirical distribution $\hnu_n := \frac{1}{n}\sum_{i=1}^n X_i$
\begin{align*}
    \P\big(\exists n\in \N^\star,\, n\Kinf\big(\hnu_n, E(\nu)\big)> \log(1/\delta) + 3\log(e\pi(1+2n))\big)\leq \delta.
\end{align*}
\end{theorem}
\todoPi{Check and prove}
Thanks to this deviation inequality we can define upper confidence bounds. Indeed if we have an i.i.d sample  $X_1,\ldots,X_n\sim \nu$ for
\[
U^{\Kinf}_n(\beta) = \sup \{\mu\geq \hmu_n: n\Kinf(\hnu_n,\mu) \leq \beta\}\,,
\]
with high probability $ \approx e^{-\beta}$ it holds
$U^{\Kinf}_n(\beta) \geq E(\nu)$.

\paragraph{Non-parametric UCB via Bayesian bootstrap} We will use the fact that $e^{-n\Kinf(\hnu_n,\mu)}$ used to build the previous upper confidence bound is well approximated by the tail of a judiciously chosen distribution. Note that a similar way to construct UCB of a parametric distribution is used by \citet{kaufmann12} for regret minimization in stochastic multi-armed bandits.To a given set of samples sample $X_1,\ldots,X_n\sim \nu$ we add a fake sample $X_0 = 1$ and defined the complemented sample set $X= \{X_0,X_1,\ldots,X_n\}$. Note that we can see the fake sample as a prior. Then with a sample $w = \{w_0,\ldots,w_n\}\sim \cD(1^{n+1})$ from a Dirichlet distribution of parameter $1^{n+1} = (1,\ldots,1)$ we can construct a Bayesian bootstrap sample \citep{rubin1981bayesian,hjort1991bayesian} of the mean $w.X := \sum_{i=0}^n w_i X_i$.
We define the non-parametric Bayesian UCB as the upper quantile of order $\delta$ of the distribution of the Bayesian bootstrap samples. Precisely we set
\[
U^{\Bayes}_n(\beta) \text{ such that } \P_{w\sim\cD(1^{n+1})} \big(w.X \geq U^{\Bayes}_n(\beta)
\big) = e^{-\beta}\]
Surprisingly we can relate this upper confidence bound with the one previously introduced.
`\begin{lemma} It holds almost surely
  \[
  ???  \leq U^{\Bayes}_n(\beta) \leq \brU^{\Kinf}_n(\beta)
  \]
  where we recall/define $\bnu_n = \frac{n}{n+1} \hnu^n + \frac{1}{n+1} \delta_1$
\begin{align*}
  U^{\Kinf}_n(\beta) &= \sup \{\mu\geq E(\hnu_n):\ n\Kinf(\hnu_n,\mu) \leq \beta\}\\
    \brU^{\Kinf}_n(\beta) &= \sup \{\mu\geq E(\bnu_n):\ (n+1)\Kinf(\bnu_n,\mu) \leq \beta\}\\
  \brU^{\Bayes}_n(\beta)  &\text{ such that } \P_{w\sim\cD(1^{n+1})} \big(w.X \geq U^{\Bayes}_n(\beta)
  \big) = e^{-\beta}\,.
\end{align*}
\end{lemma}
\todoPi{The lower bound needed to be checked}
\begin{remark}
  We can easily approximate the quantile  $U^{\Bayes}_n(\beta)$ by the quantile of a finite but large number of Bayesian bootstrap samples. Note that since if $v_0,\ldots,v_n \sim \cE(1)$ then $\big(\frac{v_0}{\sum_i v_i},\ldots, \frac{v_0}{\sum_i v_i}\big) \sim \cD(1^{n+1})$ we can generate a Bayesian bootstrap sample $w.X$ with only one pass on the sequence $X$ without the need to know in advance the length of $X$!
\end{remark}

\paragraph{Deviation inequality for Dirichlet distribution}

\begin{lemma}[Lower bound tail Dirichlet boundary crossing]
 % \label{lem:lb_tail_dirichlet}
  Consider a vector $x=(x_0,\ldots,x_n)$ of elements $\forall i \in [n+1], x_i \in [0,1]$ in the unit interval and the first element equals to $x_0=1$. Furthermore we assume that the $(x_i)_{i>0}$ take at most $S$ different values $(y_s)_{s\in[S]}$. We recall the empirical distribution $\hnu_n = \frac{1}{n}\sum_{i=1}^n \delta_{x_i}$. Then for all $E(\hnu_n)\leq \mu< 1$,
  \[
\cP_{w\sim \cD(1^{n+1})} (w.x \geq \mu ) \geq e^{-n \Kinf(\hnu_n,\mu)-S\log(n+1)}\,.
  \]
\end{lemma}
\todoPi{Can we shave the $S\log(n+1)$ factor? Maybe play with the prior}
\begin{proof}
We denote by $n_s =  \#\{i :\ x_i = y_s\}$. Without loss of generality we assume that for all $s\in[S']$ there is a sample with value $y_s$ that is $n_s>0$ and that $n_s = 0 $ for all $s>S'$. And we define $y_0=1$ and the vector $y = (y_0,\ldots,y_{S'})$. If we denote $\omega^\star$ an element in $\Sigma_{S'+1}$ such that $\omega^\star.y >\mu$ we know that $\{\omega_s \leq \omega^\star_s ,\,\forall S'>s>0 \} \subset \{\omega . y > \mu\}$.
Thus using this inlcusion and the density of the Dirichlet distribution we get
\begin{align*}
  \cP_{w\sim \cD(1^{n+1})} (w.x \geq \mu ) &= \cP_{\omega\sim \cD(1,n_1,\ldots,n_{S'})} (\omega.y \geq \mu )\\
  &\geq \cP_{\omega\sim \cD(1,n_1,\ldots,n_{S'})} (\omega_s \leq \omega^\star_s,\, \forall 0<s\leq S')\\
  &= \int_{\omega_s = 0:\ 0<s\leq S'}^{\omega^\star_s} \prod_{s\in[S']} \omega_s^{n_s-1}\left(1-\sum_{s=1}^{S'}\omega_s\right)^{1-1}\frac{\Gamma(n+1)}{\Gamma(1)\prod_{s=1}^{S'}\Gamma(n_s)}\diff \omega\\
  &= \frac{n!}{\prod_{s=1}^{S'}(n_s-1)!} \prod_{s=1}^{S'} \frac{(\omega^\star_s)^{n_s}}{n_s}\\
  & = {n\choose (n_s)_{s\in[S']}} e^{\sum_{s=1}^{S'} n_s \log(\omega_s^\star)}\\
  &\geq \frac{1}{(n+1)^{S'}} e^{n H(\homega)}e^{-n KL(\homega,\omega^\star)-nH(\homega)}\,,
\end{align*}
where we used inequality from Theorem 11.1.3 by \citet{cover2006elements}, defined the distribution $\homega = (n_1/n,\ldots,n_{S'}/n)$ and the entropy $H(\omega) = \sum_{s=1}^{S'}w_s \log(1/\omega_s)$. To conclude it remains to check that for $\lambda^\star$ that realizes the variationnal formula (Lemma~\ref{lem:var_form_Kinf})
\begin{align*}
  \Kinf(\hnu,\mu) = \frac{1}{n}\sum_{i=1}^n \log(1-\lambda^\star(x_i-\mu) ) =  \frac{1}{n}\sum_{s=1}^{S'} n_s\log(1-\lambda^\star(y_s-\mu) ) = \KL(\homega,\omega^\star)\,,
\end{align*}
for the particular choice $\omega^\star_s = \frac{n_s}{n}\frac{1}{1-\lambda^\star(y_i-\mu)}$ for $s>0$ and $\omega_0 =1- \sum_{s>0}\omega^\star_s$. It can be checked thanks to the choice of $\lambda^\star$ that $\omega^\star \in \Sigma_{S'+1}$ (see Lemma~\ref{lemma:factsH}).
\end{proof}

\paragraph{Technical results}
Note that the minimal Kullback-Leibler divergence admits a variationnal formula which will be useful in the next proofs.
\begin{lemma}[Lemma 18 by \citet{garivier2018kl}]
\label{lem:var_form_Kinf} For all $\nu \in \cP[0,1]$ and $\mu\in (0,1)$,
\[
\Kinf(\nu,u) = \max_{\lambda \in[0,1]} \E_{X\sim \nu}\left[ \log\left( 1-\lambda \frac{X-u}{1-u}\right)\right]\,,
 \]
 moreover if we denote by $\lambda^\star$ the value at which the above maximum is reached, then
 \[
   \E_{X\sim \nu} \left[\frac{1}{1-\lambda^\star(X-u)/(1-u)}\right] \leq 1\,.
 \]
\end{lemma}
Let $X$ denote a random variable with distribution $\nu \in \pset$.
We recall that $\mu \in (0,1)$.
The following function is well defined:
\[
H : \lambda \in [0,1] \longmapsto \E_{X\sim\nu}\Bigg[ \ln \! \bigg(1 - \lambda \frac{X - \mu}{1 - \mu}\bigg) \Bigg] \in \mathbb{R} \cup \{-\infty\}\,.
\]
Indeed, since $X \in [0,1]$, the random variable $\log \big(1 - \lambda(X - \mu)/(1 - \mu)\big)$ is bounded from above by
$\log \big(1+\lambda \mu /(1-\mu) \big)$. Hence, $H$ is well defined.
For $\lambda \in [0,1)$, the considered random variable is bounded from below
by $\log(1-\lambda)$, hence $H$ takes finite values. For $\lambda = 1$, we possibly have that
$H(1)$ equals $-\infty$ (this is the case in particular when $\nu\{1\} > 0$).

We begin by a study of the function $H$. \medskip

\begin{lemma}
\label{lemma:factsH}
Assume $\mu \in (0,1)$.
The function $H$ is continuous and strictly concave on $[0,1]$,
differentiable at least on $[0,1)$,
and its derivative $H'(1)$ can be defined at~$1$, with $H'(1) \in \R \cup \{ - \infty \}$.
We have the closed-form expression: for all $\lambda \in [0,1]$,
\begin{equation}\label{eq:h'}
H'(\lambda) =
- \E \Bigg[ \bigg(\frac{X- \mu}{1 - \mu} \bigg)\frac{1}{1 - \lambda \frac{X-\mu}{1 - \mu}} \Bigg]
=
\frac{1}{\lambda}
\Bigg( 1 - \E \Bigg[  \frac{1}{1 - \lambda \frac{X- \mu}{1 - \mu}}\Bigg] \Bigg)\,.
\end{equation}
It reaches a unique maximum over $[0,1]$, denoted by $\lambda^\star$,
\[
\argmax_{0 \leq \lambda \leq 1} H(\lambda) = \{ \lambda^\star \}\,.
\]
Moreover, under the additional condition $E(\nu) < \mu$, it holds $\lambda^\star > 0$ at which $H'(\lambda^\star) = 0$ if $\lambda^\star \in (0,1)$
and $H'(\lambda^\star) \geq 0$ if $\lambda^\star = 1$. In particular, $\nu\{1\} = 0$ in the case $\lambda^\star = 1$.
\end{lemma}
Note that $\Kinf(\nu,\mu) = 0$ when $\mu \leq E(\nu)$. In this case,
necessarily $\lambda^\star = 0$ (there is a unique maximum) and we still have
\[
\E \Bigg[  \frac{1}{1 - \lambda^\star \frac{X- \mu}{1 - \mu}}\Bigg] = 1\,.
\]
